# Supplementary material for: Lattice dielectric properties of rutile $\mathrm{TiO}_2$: First-principles anharmonic self-consistent phonon study
Source: arXiv:2210.15873 source file (2022-10-28)
Supplement: Supplementary file 1 [file additional_peak.tex]

\documentclass[multi=tabular,varwidth=false]{standalone}
\usepackage[numbers]{natbib}
\begin{document}
% ----- 表:born effective charges ------
\renewcommand{\arraystretch}{1.5}
{\tabcolsep = 0.15cm
  \begin{tabular}{lccc}
   \hline\hline
     Mode     & $\mathrm{r}^2$SCAN & FPSQ~\cite{gervais1974Temperature}    & FPSQ~\cite{schoche2013Infrared}\\
   \hline 
   $\epsilon_{x,1}$ & 563 & $585$ & $556\pm 5$ \\ 
%   $\epsilon_{x,2}$ &     &       & $781\pm 15$ \\ 
   $\epsilon_{z,1}$ & 598 & $592$ & $587\pm 12$ \\ 
%   $\epsilon_{z,1}$ &     &       & $710\pm 18$ \\ 
    \hline
   \hline
  \end{tabular}
}
\renewcommand{\arraystretch}{1.0}

\ifstandalone 
\input{../ver_0_after.bbl}
\fi
\end{document}
